# Supplementary material for: Fr\'echet Wavelet Distance: A Domain-Agnostic Metric for Image Generation
Source: arXiv:2312.15289 source file (2025-03-02)
Supplement: Supplementary file 1 [file fwt.tex]

\documentclass[crop,tikz]{standalone}% 'crop' is the default for v1.0, before it was 'preview'
\usepackage{amsmath}

%\usetikzlibrary{...}% tikz package already loaded by 'tikz' option
\begin{document}
\begin{tikzpicture}
  \node[draw, rectangle] at (0,0) (x){$\mathbf{x}$};

  % upper arm
  \node[draw, rectangle] at (1,  1)   (hl){$\mathbf{H_\mathcal{L}}\; \downarrow_2$};
  \node[draw, rectangle] at (2,  1.75) (hhh){$\mathbf{H_\mathcal{L}} \; \downarrow_2$};
  \node[draw, rectangle] at (2,  0.25) (hll){$\mathbf{H_\mathcal{H}} \; \downarrow_2$};

  % lower arm
  \node[draw, rectangle] at (1,  -1.) (hh){$\mathbf{H_\mathcal{H}}\; \downarrow_2$ };
  \node[draw, rectangle] at (3.4, -1.0) (b0){$\mathbf{c}_{\mathcal{H},1}$};
  \node[draw, rectangle] at (3.4,  0.25) (b2){$\mathbf{c}_{\mathcal{H},2}$};
  \node[draw, rectangle] at (3.4,  1.75) (b3){$\mathbf{c}_{\mathcal{L},2}$};

  \node[draw, rectangle] at (5,  1.75)  (fhh){$\uparrow_2 \; \mathbf{F_\mathcal{L}}$};
  \node[draw, rectangle] at (5,  0.25)  (fll){$\uparrow_2 \; \mathbf{F_\mathcal{H}}$};

  \node[draw, rectangle] at (6, -1.0) (fh){$\uparrow_2 \; \mathbf{F_\mathcal{H}}$};
  \node[draw, rectangle] at (6,  1.) (fl){$\uparrow_2 \; \mathbf{F_\mathcal{L}}$};
  \node[draw, rectangle] at (7, 0) (xhat){$\hat{\mathbf{x}}$};

  % analysis
  \draw[->] (x) |- (hh);
  \draw[->] (x) |- (hl);
  \draw[->] (hl) |- (hhh);
  \draw[->] (hl) |- (hll);

  \draw[->] (hhh) -- (b3);
  \draw[->] (hll) -- (b2);
  \draw[->] (b2) -- (fll);
  \draw[->] (hh) -- (b0);
  \draw[->] (b0) -- (fh);

  % dotted
  \draw[dotted, ->] (b3) -- (fhh);

  % synthesis
  \draw[->] (fll) -| (fl);
  \draw[->] (fhh) -| (fl);

  \draw[->] (fl) -| (xhat);
  \draw[->] (fh) -| (xhat);

  % \draw (0,0) -- (10,10); % ...
\end{tikzpicture}
\end{document}
