# Supplementary material for: Fr\'echet Wavelet Distance: A Domain-Agnostic Metric for Image Generation
Source: arXiv:2312.15289 source file (2025-03-02)
Supplement: Supplementary file 2 [file fwt_2d.tex]

\documentclass[crop,tikz]{standalone}% 'crop' is the default for v1.0, before it was 'preview'
\usepackage{amsmath}

%\usetikzlibrary{...}% tikz package already loaded by 'tikz' option
\begin{document}
\begin{tikzpicture}
  \node[draw, rectangle] at (0,0) (x){$\mathbf{x}$};

  % upper arm
  \node[draw, rectangle] at (1,  1)   (hl){$\mathbf{H_\mathcal{L}}\; \downarrow_2$};
  \node[draw, rectangle] at (2,  1.75) (hhh){$\mathbf{H_\mathcal{L}} \; \downarrow_2$};
  \node[draw, rectangle] at (2,  0.25) (hll){$\mathbf{H_\mathcal{H}} \; \downarrow_2$};

  % lower arm
  \node[draw, rectangle] at (1,  -1.) (hh){$\mathbf{H_\mathcal{H}}\; \downarrow_2$ };
  \node[draw, rectangle] at (3.4, -1.0) (b0){$\mathbf{c}_{\mathcal{H},1}$};
  \node[draw, rectangle] at (3.4,  0.25) (b2){$\mathbf{c}_{\mathcal{H},2}$};
  \node[draw, rectangle] at (3.4,  1.75) (b3){$\mathbf{c}_{\mathcal{L},2}$};

  \node[draw, rectangle] at (5,  1.75)  (fhh){$\uparrow_2 \; \mathbf{F_\mathcal{L}}$};
  \node[draw, rectangle] at (5,  0.25)  (fll){$\uparrow_2 \; \mathbf{F_\mathcal{H}}$};

  \node[draw, rectangle] at (6, -1.0) (fh){$\uparrow_2 \; \mathbf{F_\mathcal{H}}$};
  \node[draw, rectangle] at (6,  1.) (fl){$\uparrow_2 \; \mathbf{F_\mathcal{L}}$};
  \node[draw, rectangle] at (7, 0) (xhat){$\hat{\mathbf{x}}$};

  % analysis
  \draw[->] (x) |- (hh);
  \draw[->] (x) |- (hl);
  \draw[->] (hl) |- (hhh);
  \draw[->] (hl) |- (hll);

\end{tikzpicture}
\end{document}
