# Supplementary material for: Fr\'echet Wavelet Distance: A Domain-Agnostic Metric for Image Generation
Source: arXiv:2312.15289 source file (2025-03-02)
Supplement: Supplementary file 3 [file packets_1d.tex]

\documentclass[crop,tikz]{standalone}% 'crop' is the default for v1.0, before it was 'preview'
\usepackage{amsmath}
%\usetikzlibrary{...}% tikz package already loaded by 'tikz' option
\begin{document}
\begin{tikzpicture}
  \node[draw, rectangle] at (0,0) (x){$\mathbf{x}$};

  % upper arm
  \node[draw, rectangle] at (1,   2)   (hl){$\mathbf{H_\mathcal{L}}\; \downarrow_2$};
  \node[draw, rectangle] at (2,  3) (hhh){$\mathbf{H_\mathcal{L}} \; \downarrow_2$};
  \node[draw, rectangle] at (2,  1) (hll){$\mathbf{H_\mathcal{H}} \; \downarrow_2$};

  % lower arm
  \node[draw, rectangle] at (1,  -2.) (hh){$\mathbf{H_\mathcal{H}}\; \downarrow_2$ };
  \node[draw, rectangle] at (2, -1) (hph){$\mathbf{H_\mathcal{L}} \downarrow_2$};
  \node[draw, rectangle] at (2, -3) (hpl){$\mathbf{H_\mathcal{H}} \downarrow 2$};

  \node[draw, rectangle] at (4, -3) (b0){$\mathbf{c}_{\mathcal{H},\mathcal{H}}$};
  \node[draw, rectangle] at (4, -1) (b1){$\mathbf{c}_{\mathcal{H},\mathcal{L}}$};
  \node[draw, rectangle] at (4,  1) (b2){$\mathbf{c}_{\mathcal{L},\mathcal{H}}$};
  \node[draw, rectangle] at (4,  3) (b3){$\mathbf{c}_{\mathcal{L},\mathcal{L}}$};

  \node[draw, rectangle] at (6, 3)  (fhh){$\uparrow_2 \; \mathbf{F_\mathcal{L}}$};
  \node[draw, rectangle] at (6, 1)  (fll){$\uparrow_2 \; \mathbf{F_\mathcal{H}} $};
  \node[draw, rectangle] at (6, -1) (fph){$\uparrow_2 \; \mathbf{F_\mathcal{L}} $};
  \node[draw, rectangle] at (6, -3) (fpl){$\uparrow_2 \; \mathbf{F_\mathcal{H}} $};

  \node[draw, rectangle] at (7, -2.0) (fh){$\uparrow_2 \; \mathbf{F_\mathcal{H}}$ };
  \node[draw, rectangle] at (7,  2.) (fl){$\uparrow_2 \; \mathbf{F_\mathcal{L}}$};
  \node[draw, rectangle] at (8, 0) (xhat){$\hat{\mathbf{x}}$};

  % analysis
  \draw[->] (x) |- (hh);
  \draw[->] (x) |- (hl);
  \draw[->] (hl) |- (hhh);
  \draw[->] (hl) |- (hll);
  \draw[->] (hh) |- (hph);
  \draw[->] (hh) |- (hpl);

  \draw[->] (hhh) -- (b3);
  \draw[->] (hll) -- (b2);
  \draw[->] (hph) -- (b1);
  \draw[->] (hpl) -- (b0);

  % dotted
  \draw[dotted, ->] (b3) -- (fhh);
  \draw[dotted, ->] (b2) -- (fll);
  \draw[dotted, ->] (b1) -- (fph);
  \draw[dotted, ->] (b0) -- (fpl);

  % synthesis
  \draw[->] (fll) -| (fl);
  \draw[->] (fhh) -| (fl);
  \draw[->] (fpl) -| (fh);
  \draw[->] (fph) -| (fh);

  \draw[->] (fl) -| (xhat);
  \draw[->] (fh) -| (xhat);

  % \draw (0,0) -- (10,10); % ...
\end{tikzpicture}
\end{document}
