# Supplementary material for: Fr\'echet Wavelet Distance: A Domain-Agnostic Metric for Image Generation
Source: arXiv:2312.15289 source file (2025-03-02)
Supplement: Supplementary file 4 [file packets_2d.tex]

\documentclass[crop,tikz]{standalone}% 'crop' is the default for v1.0, before it was 'preview'
\usepackage{amsmath}
%\usetikzlibrary{...}% tikz package already loaded by 'tikz' option
\begin{document}
\begin{tikzpicture}
  \node[draw, rectangle] at (0,0)   (I){$\mathbf{X}$};

  % 1st lvl filters
  \node[draw, rectangle] at (-4.25, -1) (Ha){$\mathbf{H_a}\downarrow_2$};
  \node[draw, rectangle] at (-1, -1) (Hz){$\mathbf{H_h}\downarrow_2$};
  \node[draw, rectangle] at ( 1, -1) (Hv){$\mathbf{H_v}\downarrow_2$};
  \node[draw, rectangle] at ( 2.5, -1) (Hd){$\mathbf{H_d}\downarrow_2$};

  % 1st lvl image filter arrows.
  \draw[->] (I) -| (Ha);
  \draw[->] (I) -| (Hz);
  \draw[->] (I) -| (Hv);
  \draw[->] (I) -| (Hd);

  % 1st lvl coefficients.
  \node[draw, rectangle] at (-4.25, -2) (a){$\mathbf{p}_a$};
  \node[draw, rectangle] at (-1, -2) (z){$\mathbf{p}_h$};
  \node[draw, rectangle] at ( 1, -2) (v){$\mathbf{p}_v$};
  \node[draw, rectangle] at ( 2.5, -2) (d){$\mathbf{p}_d$};

  % 1st lvl coefficient arrows.
  \draw[->] (Ha) -- (a);
  \draw[->] (Hz) -- (z);
  \draw[->] (Hv) -- (v);
  \draw[->] (Hd) -- (d);

  % 2nd lvl filters.
  \node[draw, rectangle] at (-6.5, -3) (Haa){$\mathbf{H_a} \downarrow_2$};
  \node[draw, rectangle] at (-5, -3) (Haz){$\mathbf{H_h} \downarrow_2$};
  \node[draw, rectangle] at (-3.5, -3) (Hav){$\mathbf{H_v} \downarrow_2$};
  \node[draw, rectangle] at (-2, -3) (Had){$\mathbf{H_d} \downarrow_2$};

  \node[draw, rectangle] at (-6.5,  -3.75) (aa){$\mathbf{p}_{a,a}$};
  \node[draw, rectangle] at (-5,  -3.75) (az){$\mathbf{p}_{a,h}$};
  \node[draw, rectangle] at (-3.5,-3.75) (av){$\mathbf{p}_{a,v}$};
  \node[draw, rectangle] at (-2,  -3.75) (ad){$\mathbf{p}_{a,d}$};

  % 2nd lvl coefficient arrows.
  \draw[->] (Haa) -- (aa);
  \draw[->] (Haz) -- (az);
  \draw[->] (Hav) -- (av);
  \draw[->] (Had) -- (ad);

  \draw[->] (a) -| (Haa);
  \draw[->] (a) -| (Haz);
  \draw[->] (a) -| (Hav);
  \draw[->] (a) -| (Had);

  % 2nd lvl inverse filters
  \node[draw, rectangle] at (-6.5,  -6) (Faa){$ \uparrow_2 \mathbf{F_a}$};
  \node[draw, rectangle] at (-5, -6) (Faz){$ \uparrow_2 \mathbf{F_h}$  };
  \node[draw, rectangle] at (-3.5, -6) (Fav){$ \uparrow_2 \mathbf{F_v}$};
  \node[draw, rectangle] at (-2,   -6) (Fad){$ \uparrow_2 \mathbf{F_d}$};
  
  % analysis - synthesis arrows
  \draw[->, dashed] (aa) -- (Faa);
  \draw[->, dashed] (az) -- (Faz);
  \draw[->, dashed] (av) -- (Fav);
  \draw[->, dashed] (ad) -- (Fad);

  % 1st lvl filters
  \node[draw, rectangle] at (-4.25,-7) (Fa){$\uparrow_2 \mathbf{F_a}  $};
  \node[draw, rectangle] at (-1,  -7) (Fz){$\uparrow_2 \mathbf{F_h} $};
  \node[draw, rectangle] at ( 1,  -7) (Fv){$\uparrow_2 \mathbf{F_v} $};
  \node[draw, rectangle] at ( 2.5,  -7) (Fd){$\uparrow_2 \mathbf{F_d} $};

  % 1st lvl arrows
  \draw[->] (Faa) |- (Fa);
  \draw[->] (Faz) |- (Fa);
  \draw[->] (Fav) |- (Fa);
  \draw[->] (Fad) |- (Fa);

  \draw[->, dashed] (z) -- (Fz);
  \draw[->, dashed] (v) -- (Fv);
  \draw[->, dashed] (d) -- (Fd);

  \node[draw, rectangle] at (0,-8)   (hI){$\hat{\mathbf{X}}$};

  \draw[->] (Fa) |- (hI);
  \draw[->] (Fz) |- (hI);
  \draw[->] (Fv) |- (hI);
  \draw[->] (Fd) |- (hI);

\end{tikzpicture}
\end{document}
